# Supplementary material for: Inertial spin dynamics in epitaxial cobalt films
Source: arXiv:2109.03076 ancillary file (2021-09-11)
Supplement: Supplementary file 1 [file InertialSpinDynamicsInEpitaxialCobaltFilms_SM.pdf]

# Inertial spin dynamics in epitaxial cobalt films

Vivek Unikandanunni,[1] Rajasekhar Medapalli,[2,3] Marco Asa,[4] Edoardo Albisetti,[4]
Daniela Petti,[4] Riccardo Bertacco,[4] Eric E. Fullerton,[2] and Stefano Bonetti[1,5,*]

[1] *Department of Physics, Stockholm University, 10691 Stockholm, Sweden*
[2] *Center for Memory and Recording Research, University of California San Diego, San Diego, CA 92093, USA*
[3] *Department of Physics, School of Sciences, National Institute of Technology, Andhra Pradesh-534102, India*
[4] *Department of Physics, Politecnico di Milano Technical University, Milano, Italy*
[5] *Department of Molecular Sciences and Nanosystems, Ca' Foscari University of Venice, 30172 Venice, Italy*

## I. MAGNETIC SAMPLE CHARACTERIZATION

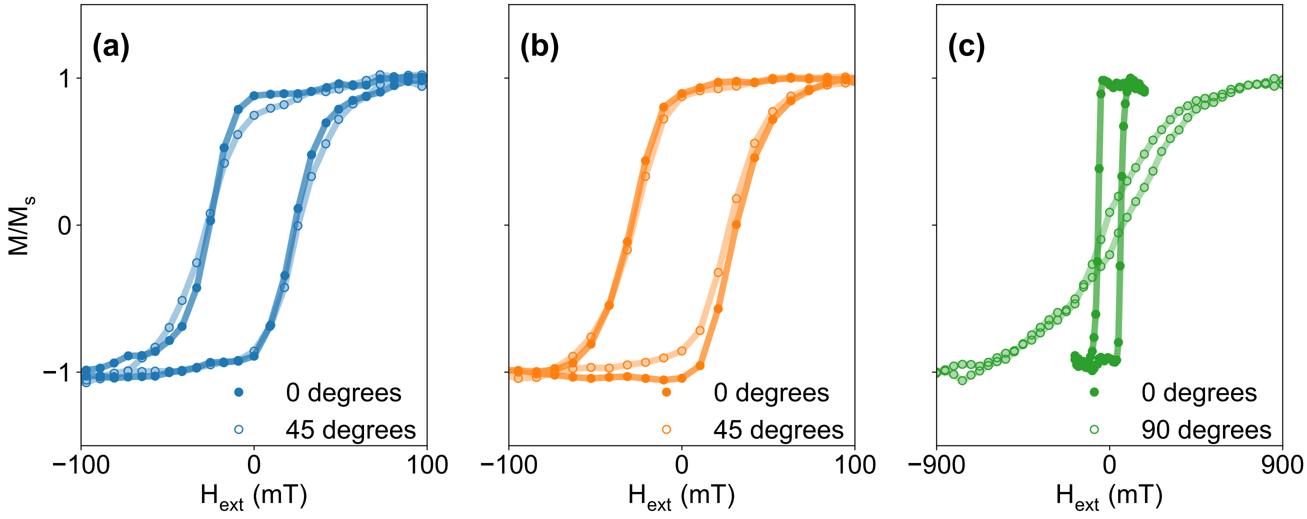


FIG. 1. MOKE magnetometry characterization of the three samples, showing the easy and hard magnetization axes loops. For the cubic samples (a) fcc and (b) bcc, the easy axis is the [100] crystalline direction, with the [110] being the nominal hard axis. For the (c) hcp sample, the easy axis is in plane and along the $c$-axis [0001], and the hard axis is orthogonal to it, within the sample plane.

---

* stefano.bonetti@fysik.su.se

## II. STRUCTURAL SAMPLE CHARACTERIZATION

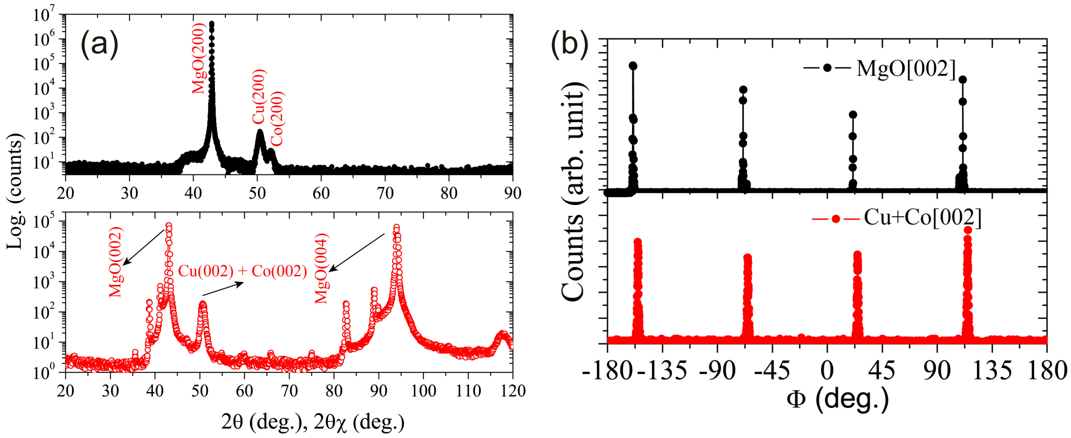


FIG. 2. XRD characterization of the epitaxial fcc cobalt sample. The sample stack from top surface to bottom one is Pt(3 nm)/Co(15 nm)/Cu(20 nm)/MgO (substrate). The 3-nm-thick Pt layer is the capping layer and copper layer is the seed layer for epitaxial growth. (a) $2\theta$ and $2\theta\chi$ scan for out-of-plane and (b) $\phi$ scans for in-plane crystallographic characterizations.

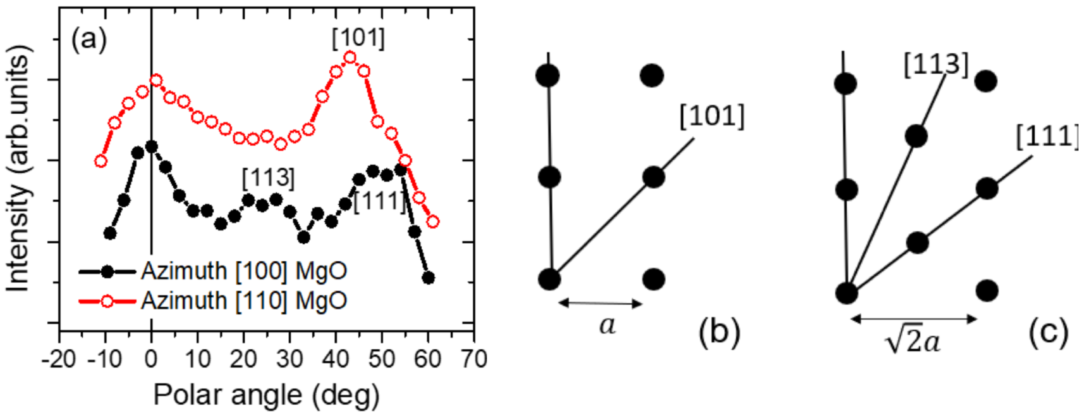


FIG. 3. Structural characterization of the epitaxial bcc sample. (a) XPD curves of Co 2p3/2 along the [100] (black dots, bottom) and [110] (red empty dots, top) azimuths of the substrate; (b),(c) Atomic arrangement in the (010) and (110) planes of a bcc structure. An MgO (001) crystal has been introduced into ultra-high vacuum and annealed at 600 °C for 1 hour to remove water and surface contaminants. Cobalt (8 nm) has been deposited at room temperature from a high purity metal rod by Molecular Beam Epitaxy (MBE) with a deposition rate of 2 Å/min at a pressure lower than $7.5 \cdot 10^{-8}$ Pa. Afterwards, the sample has been annealed at 250 °CC for 20 minutes to improve its crystalline quality. Crystal order of the Co film has been assessed by means of in situ X-Ray Photoemission Diffraction (XPD). The Co 2p3/2 photoemission peaks excited by Al-K$\alpha$ radiation were recorded by scanning the polar angle along the [100] and [110] azimuths of the MgO Substrate.

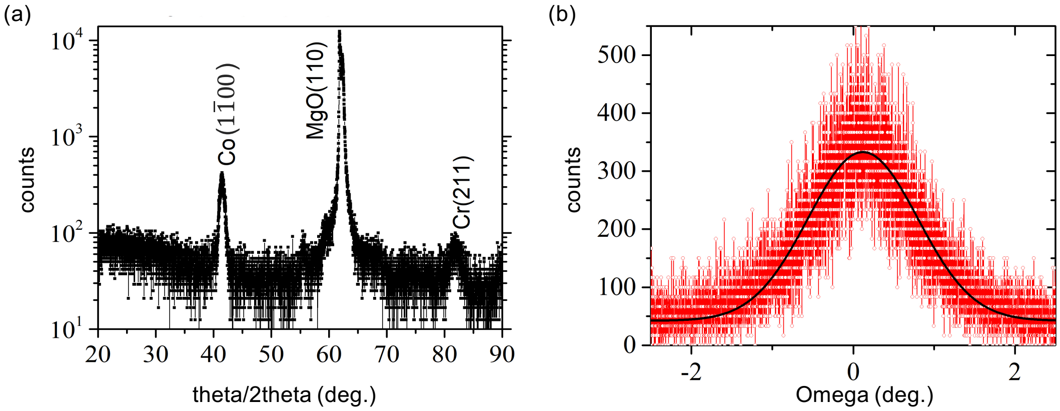


FIG. 4. XRD characterization of the epitaxial hcp cobalt sample. A 10-nm-thick epitaxial hcp(1-100)-cobalt thin film was grown as Co[1-100] on a MgO(110) substrate and a Cr(211) seed layer. The Co layer was capped with a 3-nm-thick Pt layer. The easy axis of magnetization is along the *c*-axis [0001] and lies in the plane of the film. (a) 2  scan for out of plane characterization. (b) Rocking curve of cobalt layer for in plane characterization. The FWHM of the rocking curve is about 1.5 degree.

## III. SUPPLEMENTAL PUMP-PROBE MEASUREMENTS

### A. Pump field polarization dependence

Fig. 5 show the same measurement on the hcp sample presented in the main text with $H_{THz}$ perpendicular to the magnetization, together with the data taken when $H_{THz}$ is parallel to it. Both coherent precession and nutation oscillations disappear in the latter case, while the incoherent demagnetization is still present, due to the energy deposited in the sample by the THz pulse [1].

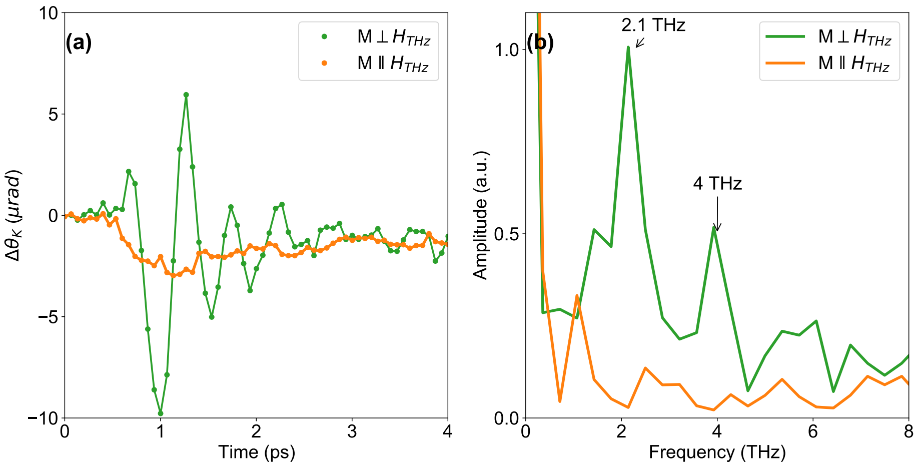


FIG. 5. (a)Time resolved magneto-optical Kerr rotation following a THz pump field with polarization perpendicular and parallel to the direction of the static magnetization. (b) Fourier transform of the time-resolved data in panel (a).

### B. Off-resonant nutation measurements

Figure 6(a) shows the magnetization dynamics triggered in fcc and hcp samples using a terahertz field with the spectrum plotted in panel (b). No phase difference between the time integral of THz pulse and the coherent precession is observed, and no nutation resonance is found.

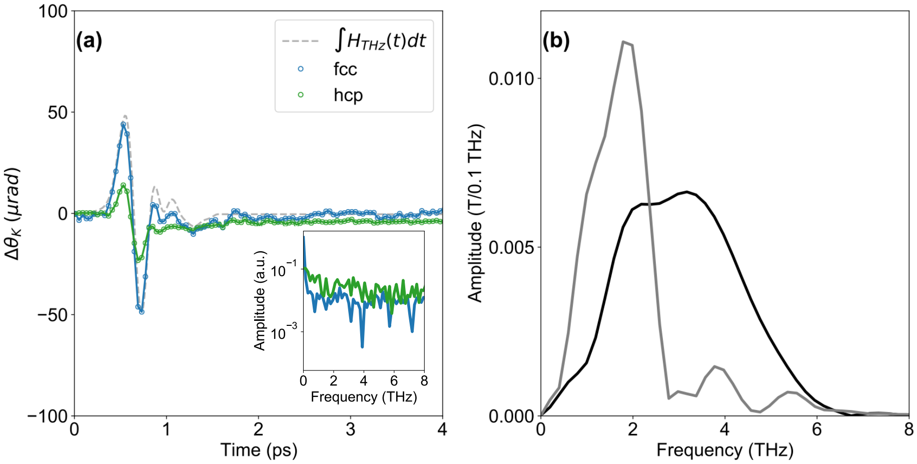


FIG. 6. (a) Time resolved magneto-optical Kerr rotation following a THz pump field generated with the organic crystal DSTMS. Inset: Fourier transform of the data in the main panel. (b) Fourier transform of the two THz pump fields generated with different nonlinear crystals used in this work.

[1] S. Bonetti, M. Hoffmann, M.-J. Sher, Z. Chen, S.-H. Yang, M. Samant, S. Parkin, and H. Dürr, Thz-driven ultrafast spin-lattice scattering in amorphous metallic ferromagnets, Physical review letters **117**, 087205 (2016).
